# Supplementary material for: Testing-driven Variable Selection in Bayesian Modal Regression
Source: arXiv:2510.23831 ancillary file (2025-10-27)
Supplement: Supplementary file 1 [file Supplementary_materials_for_Testing-driven_Variable_Selection_in_Bayesian_Modal_Regression_Arxiv.pdf]

# Supplementary Materials for "Testing-driven Variable Selection in Bayesian Modal Regression" by Duan et al.

*This supplement is a preprint under review.*

# Web Appendix: Updates for model parameters in the EM algorithm

The updates for $\beta_0$, $\nu$, and $\gamma$ are obtained via numerical optimization of the corresponding objective functions presented below, and the update for $\theta$ is in a closed form given next. For $k \geq 0$,

$$
\begin{aligned}
\beta_0^{(k+1)} &= \arg\max_{\beta_0 \in \mathbb{R}} Q\left(\beta_0, \boldsymbol{\beta}^{(k+1)}, \nu^{(k)}, \gamma^{(k)}, \theta^{(k)} \mid \boldsymbol{\beta}^{(k+1)}, \beta_0^{(k)}, \nu^{(k)}, \gamma^{(k)}, \theta^{(k)}\right) \\
&= \arg\max_{\beta_0 \in \mathbb{R}} \Bigg[ -\frac{\beta_0^2}{2 \times 10^6} - \frac{\nu^{(k)}+1}{2} \sum_{i=1}^{n} \log\Big\{1 + \frac{(y_i - \beta_0 - \boldsymbol{x}_i\boldsymbol{\beta}^{(k+1)})^2}{\nu^{(k)}} \\
&\quad \times \gamma^{(k)2\left\{-\mathbb{1}_{[0,+\infty)}(y_i-\beta_0-\boldsymbol{x}_i\boldsymbol{\beta}^{(k+1)})+\mathbb{1}_{(-\infty,0)}(y_i-\beta_0-\boldsymbol{x}_i\boldsymbol{\beta}^{(k+1)})\right\}}\Big\}\Bigg], \\
\nu^{(k+1)} &= \arg\max_{\nu \in \mathbb{R}^+} Q\left(\nu, \boldsymbol{\beta}^{(k+1)}, \beta_0^{(k+1)}, \gamma^{(k)}, \theta^{(k)} \mid \boldsymbol{\beta}^{(k+1)}, \beta_0^{(k+1)}, \nu^{(k)}, \gamma^{(k)}, \theta^{(k)}\right) \\
&= \arg\max_{\nu \in \mathbb{R}^+} \Bigg[ -\frac{(\log\nu - 1)^2}{2} - (\frac{n}{2}+1)\log\nu + n\log(\frac{\Gamma(\frac{\nu+1}{2})}{\Gamma(\frac{\nu}{2})}) \\
&\quad - \frac{\nu+1}{2} \sum_{i=1}^{n} \log\Big\{1 + \frac{\left(y_i - \beta_0^{(k+1)} - \boldsymbol{x}_i\boldsymbol{\beta}^{(k+1)}\right)^2}{\nu} \\
&\quad \gamma^{(k)2\left\{-\mathbb{1}_{[0,+\infty)}(y_i-\beta_0^{(k+1)}-\boldsymbol{x}_i\boldsymbol{\beta}^{(k+1)})+\mathbb{1}_{(-\infty,0)}(y_i-\beta_0^{(k+1)}-\boldsymbol{x}_i\boldsymbol{\beta}^{(k+1)})\right\}}\Big\}\Bigg], \\
\gamma^{(k+1)} &= \arg\max_{\gamma \in \mathbb{R}^+} Q\left(\gamma, \boldsymbol{\beta}^{(k+1)}, \beta_0^{(k+1)}, \nu^{(k+1)}, \theta^{(k)} \mid \boldsymbol{\beta}^{(k+1)}, \beta_0^{(k+1)}, \nu^{(k+1)}, \gamma^{(k)}, \theta^{(k)}\right) \\
&= \arg\max_{\gamma \in \mathbb{R}^+} \Bigg[ (n+c-1)\log\gamma - n\log(\gamma^2+1) - d\gamma
\end{aligned}
$$

$$
-\frac{\nu^{(k+1)}+1}{2}\sum_{i=1}^{n}\log\Big\{1+\frac{\left(y_i-\beta_0^{(k+1)}-\boldsymbol{x}_i\boldsymbol{\beta}^{(k+1)}\right)^2}{\nu^{(k+1)}}
$$

$$
\gamma^{2\left\{-\mathbb{1}_{[0,+\infty)}(y_i-\beta_0^{(k+1)}-\boldsymbol{x}_i\boldsymbol{\beta}^{(k+1)})+\mathbb{1}_{(-\infty,0)}(y_i-\beta_0^{(k+1)}-\boldsymbol{x}_i\boldsymbol{\beta}^{(k+1)})\right\}}\Big\}\Bigg],
$$

$$
\theta^{(k+1)}=\frac{\sum_{i=1}^{p}E\left(\lambda_j\left|\beta_j^{(k+1)},\theta^{(k)},\boldsymbol{y}\right.\right)+a-1}{a+b+p-2}.
$$

The above updates are done sequentially after updating $\boldsymbol{\beta}^{(k)}$ to $\boldsymbol{\beta}^{(k+1)}$ via maximizing the objective function

$$
\sum_{i=1}^{n}\log\left\{\left(1+\frac{\varepsilon_{i,k}^2}{\gamma^{(k)2}\nu^{(k)}}\right)^{-(\nu^{(k)}+1)/2}\mathbb{1}_{[0,+\infty)}(\varepsilon_{i,k})+\left(1+\frac{\gamma^{(k)2}\varepsilon_{i,k}^2}{\nu^{(k)}}\right)^{-(\nu^{(k)}+1)/2}\mathbb{1}_{(-\infty,0)}(\varepsilon_{i,k})\right\}
$$

$$
-\sum_{j=1}^{p}\left\{\left(1-\hat{p}_j^{(k)}\right)t_0+\hat{p}_j^{(k)}t_1\right\}|\beta_j|, \tag{1}
$$

which is equation (7) in the main article that can be interpreted as a penalized/regularized log-likelihood.

Regularization not only facilitates variable selection but is also often necessary to achieve sensible inference when $p>n$. To further improve the computational efficiency of the EM algorithm in such challenging scenarios, we employ a coordinate ascent algorithm to update $\boldsymbol{\beta}$, where, instead of updating $\boldsymbol{\beta}^{(k)}$ to $\boldsymbol{\beta}^{(k+1)}$ by maximizing (1) with respect to $\boldsymbol{\beta}$, we maximize it with respect to $\beta_j$ for one $j\in\{1,\ldots,p\}$ at a time and cycle sequentially through all coordinates for $T$ (e.g., $T=2$) rounds. Because the penalty in (1) is separable, that is, the LASSO-like penalty is covariate-specific, each coordinate update can be efficiently implemented. Thus, each M-step embeds a $T$-iteration coordinate ascent update for $\boldsymbol{\beta}$. We repeat the EM iterations until the two successive updated estimates for $\Theta_{-\boldsymbol{\lambda}}$ differ by no more than $10^{-7}$ in $L_2$-norm.
